# Supplementary material for: Heptazine, Cyclazine, and Related Compounds: Chemically-Accurate Estimates of the Inverted Singlet-Triplet Gap
Source: arXiv:2310.19768 ancillary file (2023-12-06)
Supplement: Supplementary file 1 [file Heptazine-SI.pdf]

# Supporting Information for

# Heptazine, Cyclazine, and Related Compounds: Chemically-Accurate Estimates of the Inverted Singlet-Triplet Gap

Pierre-François Loos,[†] Filippo Lipparini,[‡] and Denis Jacquemin[*,¶,§]

†*Laboratoire de Chimie et Physique Quantiques, Université de Toulouse, CNRS, UPS, France*

‡*Dipartimento di Chimica e Chimica Industriale, University of Pisa, Via Moruzzi 3, 56124 Pisa, Italy*

¶*Nantes Université, CNRS, CEISAM UMR 6230, F-44000 Nantes, France*

§*Institut Universitaire de France, 75005 Paris, France*

E-mail: Denis.Jacquemin@univ-nantes.fr

## S1. BENCHMARK

**Table S1: Reference vertical transition energies for compounds 1–10. All values are in eV. The numbers in parentheses are the percentages of single excitation involved in the transition computed at the CC3/aug-cc-pVDZ level.**

| | | CCSD | | | CC3 | | | CCSDT | TBE[a] |
|---|---|---|---|---|---|---|---|---|---|
| Compound | State | 6-31+G(d) | *aug*-cc-pVDZ | *aug*-cc-pVTZ | 6-31+G(d) | *aug*-cc-pVDZ | *aug*-cc-pVTZ | 6-31+G(d) | *aug*-cc-pVTZ |
| **1** | $S_1$ | 2.829 | 2.901 | 2.953 | 2.633 | 2.693 (86.3%) | 2.708 | 2.642 | 2.717 |
| | $T_1$ | 3.017 | 3.049 | 3.087 | 2.873 | 2.898 (95.7%) | | | 2.936 |
| **2** | $S_1$ | 1.073 | 1.092 | 1.090 | 0.974 | 0.990 (87.2%) | 0.978 | 0.975 | 0.979 |
| | $T_1$ | 1.185 | 1.165 | 1.154 | 1.142 | 1.121 (96.1%) | | | 1.110 |
| **3** | $S_1$ | 1.672 | 1.703 | 1.719 | 1.535 | 1.559 (86.9%) | 1.557 | 1.540 | 1.562 |
| | $T_1$ | 1.746 | 1.732 | 1.733 | 1.677 | 1.662 (96.1%) | | | 1.663 |
| **4** | $S_1$ | 2.294 | 2.342 | 2.374 | 2.125 | 2.164 (86.5%) | 2.169 | 2.133 | 2.177 |
| | $T_1$ | 2.377 | 2.382 | 2.394 | 2.282 | 2.284 (96.0%) | | | 2.296 |
| **5** | $S_1$ | 2.241 | 2.290 | 2.323 | 2.074 | 2.114 (86.5%) | 2.120 | 2.081 | 2.127 |
| | $T_1$ | 2.313 | 2.312 | 2.324 | 2.221 | 2.218 (96.1%) | | | 2.230 |
| **6** | $S_1$ | 0.921 | 0.932 | 0.922 | 0.841 | 0.849 (87.2%) | 0.834 | 0.840 | 0.833 |
| | $T_1$ | 0.969 | 0.944 | 0.922 | 0.949 | 0.926 (96.2%) | | | 0.904 |
| **7** | $S_1$ | 0.774 | 0.775 | 0.758 | 0.713 | 0.714 (87.1%) | 0.696 | 0.710 | 0.693 |
| | $T_1$ | 0.792 | 0.761 | 0.731 | 0.794 | 0.765 (96.2%) | | | 0.735 |
| **8** | $S_1$ | 0.627 | 0.619 | 0.594 | 0.587 | 0.580 (87.1%) | 0.560 | 0.581 | 0.554 |
| | $T_1$ | 0.634 | 0.595 | 0.558 | 0.656 | 0.620 (96.3%) | | | 0.583 |
| **9** | $S_1$ | 1.341 | 1.388 | 1.407 | 1.224 | 1.268 (86.2%) | 1.261 | 1.227 | 1.264 |
| | $T_1$ | 1.499 | 1.511 | 1.516 | 1.445 | 1.458 (95.8%) | | | 1.463 |
| **10** | $S_1$ | 1.621 | 1.666 | 1.694 | 1.477 | 1.519 (86.0%) | 1.515 | 1.484 | 1.522 |
| | $T_1$ | 1.897 | 1.907 | 1.925 | 1.798 | 1.809 (95.5%) | | | 1.827 |

[a] Theoretical best estimate obtained from CC3/*aug*-cc-pVTZ + [CCSDT/6-31+G(d) − CC3/6-31+G(d)] for $S_1$ and CC3/*aug*-cc-pVDZ + [CCSD/*aug*-cc-pVTZ − CCSD/*aug*-cc-pVDZ] for $T_1$.

**Table S2: Vertical transition energies to the lowest singlet and triplet states (and corresponding STG) obtained with various wave function approaches. All values are in eV and obtained with the *aug*-cc-pVTZ basis set.**

| | CIS(D) | | | ADC(2) | | | SOS-ADC(2) | | | SCS-ADC(2) | | | CC2 | | | SOS-CC2 | | | SCS-CC2 | | | CCSD | | |
|---|---|---|---|---|---|---|---|---|---|---|---|---|---|---|---|---|---|---|---|---|---|---|---|---|
| Compound | $S_1$ | $T_1$ | STG | $S_1$ | $T_1$ | STG | $S_1$ | $T_1$ | STG | $S_1$ | $T_1$ | STG | $S_1$ | $T_1$ | STG | $S_1$ | $T_1$ | STG | $S_1$ | $T_1$ | STG | $S_1$ | $T_1$ | STG |
| **1** | 2.659 | 3.178 | -0.519 | 2.675 | 2.921 | -0.246 | 2.893 | 3.345 | -0.452 | 2.827 | 3.206 | -0.379 | 2.767 | 3.006 | -0.239 | 2.933 | 3.382 | -0.389 | 2.883 | 3.256 | -0.373 | 2.953 | 3.087 | -0.134 |
| **2** | 1.042 | 1.319 | -0.277 | 1.001 | 1.138 | -0.137 | 1.121 | 1.394 | -0.273 | 1.084 | 1.309 | -0.225 | 1.051 | 1.181 | -0.130 | 1.137 | 1.407 | -0.270 | 1.110 | 1.330 | -0.220 | 1.090 | 1.154 | -0.064 |
| **3** | 1.600 | 1.924 | -0.324 | 1.551 | 1.664 | -0.113 | 1.713 | 1.959 | -0.246 | 1.663 | 1.863 | -0.200 | 1.615 | 1.721 | -0.106 | 1.739 | 1.980 | -0.241 | 1.700 | 1.893 | -0.193 | 1.719 | 1.733 | -0.014 |
| **4** | 2.220 | 2.683 | -0.463 | 2.159 | 2.298 | -0.139 | 2.348 | 2.626 | -0.278 | 2.291 | 2.521 | -0.230 | 2.235 | 2.366 | -0.131 | 2.384 | 2.659 | -0.275 | 2.338 | 2.563 | -0.225 | 2.374 | 2.394 | -0.020 |
| **5** | 2.139 | 2.559 | -0.420 | 2.098 | 2.225 | -0.127 | 2.289 | 2.552 | -0.263 | 2.231 | 2.447 | -0.216 | 2.178 | 2.296 | -0.118 | 2.324 | 2.581 | -0.257 | 2.279 | 2.487 | -0.208 | 2.323 | 2.324 | -0.001 |
| **6** | 0.905 | 1.163 | -0.258 | 0.851 | 0.945 | -0.094 | 0.947 | 1.165 | -0.218 | 0.918 | 1.092 | -0.174 | 0.903 | 0.988 | -0.085 | 0.969 | 1.182 | -0.213 | 0.949 | 1.116 | -0.167 | 0.922 | 0.922 | 0.000 |
| **7** | 0.772 | 0.991 | -0.219 | 0.708 | 0.782 | -0.074 | 0.781 | 0.977 | -0.196 | 0.759 | 0.912 | -0.153 | 0.762 | 0.827 | -0.065 | 0.808 | 0.999 | -0.191 | 0.794 | 0.941 | -0.147 | 0.758 | 0.731 | 0.027 |
| **8** | 0.640 | 0.829 | -0.189 | 0.565 | 0.635 | -0.070 | 0.617 | 0.808 | -0.191 | 0.602 | 0.750 | -0.148 | 0.623 | 0.681 | -0.058 | 0.650 | 0.835 | -0.185 | 0.642 | 0.783 | -0.141 | 0.594 | 0.558 | 0.036 |
| **9** | 1.286 | 1.799 | -0.513 | 1.274 | 1.488 | -0.214 | 1.141 | 1.774 | -0.633 | 1.369 | 1.680 | -0.311 | 1.343 | 1.555 | -0.212 | 1.436 | 1.803 | -0.367 | 1.407 | 1.720 | -0.313 | 1.407 | 1.516 | -0.109 |
| **10** | 1.595 | 2.262 | -0.667 | 1.639 | 2.074 | -0.435 | 1.686 | 2.189 | -0.503 | 1.639 | 2.074 | -0.435 | 1.673 | 2.119 | -0.446 | 1.706 | 2.223 | -0.517 | 1.673 | 2.119 | -0.446 | 1.694 | 1.925 | -0.231 |

**Table S3: Vertical transition energies to the lowest singlet and triplet states (and corresponding STG) obtained with various TD-DFT approaches. All values are in eV and obtained with the *aug*-cc-pVTZ basis set.**

| | PBE0-2 | | | SOS-PBE-QIDH | | | SCS-PBE-QIDH | | | SOS-RSX-QIDH | | |
|---|---|---|---|---|---|---|---|---|---|---|---|---|
| Compound | $S_1$ | $T_1$ | STG | $S_1$ | $T_1$ | STG | $S_1$ | $T_1$ | STG | $S_1$ | $T_1$ | STG |
| **1** | 2.890 | 3.053 | -0.163 | 2.733 | 2.998 | -0.265 | 2.770 | 2.987 | -0.217 | 2.573 | 2.881 | -0.308 |
| **2** | 1.122 | 1.223 | -0.101 | 1.009 | 1.170 | -0.161 | 1.039 | 1.163 | -0.124 | 0.782 | 0.905 | -0.123 |
| **3** | 1.714 | 1.761 | -0.047 | 1.590 | 1.691 | -0.101 | 1.621 | 1.685 | -0.064 | 1.398 | 1.469 | -0.071 |
| **4** | 2.351 | 2.451 | -0.100 | 2.206 | 2.344 | -0.138 | 2.239 | 2.340 | -0.101 | 2.033 | 2.154 | -0.121 |
| **5** | 2.294 | 2.337 | -0.043 | 2.154 | 2.248 | -0.094 | 2.188 | 2.245 | -0.057 | 1.981 | 2.049 | -0.068 |
| **6** | 0.965 | 1.755[a] | -0.790[a] | 0.850 | 1.203 | -0.353 | 0.881 | 1.201 | -0.320 | 0.593 | 0.921 | -0.328 |
| **7** | 0.811 | 0.880 | -0.069 | 0.695 | 0.830 | -0.135 | 0.728 | 0.825 | -0.097 | 0.409 | 0.678 | -0.269 |
| **8** | 0.659 | 0.733 | -0.074 | 0.541 | 0.676 | -0.135 | 0.574 | 0.673 | -0.099 | 0.224 | 0.495 | -0.271 |
| **9** | 1.405 | 1.711 | -0.306 | 1.268 | 1.546 | -0.278 | 1.305 | 1.538 | -0.233 | 1.046 | 1.213 | -0.167 |
| **10** | 1.675 | 1.962 | -0.287 | 1.527 | 1.916 | -0.389 | 1.566 | 1.906 | -0.340 | 1.320 | 1.748 | -0.428 |

[a] With the PBE0-2 functional, we observe a strong orbital mixing in the lowest-energy triplet state, which has therefore an unclear character. These values strongly influence the statistics.

**Table S4: MSE, MAE, and SDE (in eV) determined for the $S_0$–$S_1$ vertical transitions, considering the TBE of Table S1 as reference.**

| Method | MSE | MAE | SDE |
|---|---|---|---|
| CIS(D) | 0.043 | 0.055 | 0.043 |
| ADC(2) | 0.009 | 0.029 | 0.044 |
| SOS-ADC(2) | 0.111 | 0.135 | 0.090 |
| SCS-ADC(2) | 0.096 | 0.096 | 0.022 |
| CC2 | 0.072 | 0.072 | 0.030 |
| SOS-CC2 | 0.166 | 0.166 | 0.040 |
| SCS-CC2 | 0.135 | 0.135 | 0.026 |
| CCSD | 0.141 | 0.141 | 0.063 |
| PBE0-2 | 0.146 | 0.146 | 0.023 |
| SOS-PBE-QIDH | 0.015 | 0.017 | 0.015 |
| SCS-PBE-QIDH | 0.048 | 0.048 | 0.014 |
| SOS-RSX-QIDH | -0.207 | 0.207 | 0.063 |

**Table S5: MSE, MAE, and SDE (in eV) determined for the $S_0$–$T_1$ vertical transitions, considering the TBE of Table S1 as reference.**

| Method | MSE | MAE | SDE |
|---|---|---|---|
| CIS(D) | 0.296 | 0.296 | 0.073 |
| ADC(2) | 0.042 | 0.046 | 0.076 |
| SOS-ADC(2) | 0.304 | 0.304 | 0.056 |
| SCS-ADC(2) | 0.211 | 0.211 | 0.031 |
| CC2 | 0.099 | 0.099 | 0.069 |
| SOS-CC2 | 0.330 | 0.330 | 0.061 |
| SCS-CC2 | 0.246 | 0.246 | 0.040 |
| CCSD | 0.060 | 0.066 | 0.054 |
| PBE0-2[a] | 0.212 | 0.212 | 0.229 |
| SOS-PBE-QIDH | 0.088 | 0.088 | 0.079 |
| SCS-PBE-QIDH | 0.082 | 0.082 | 0.080 |
| SOS-RSX-QIDH | -0.123 | 0.127 | 0.084 |

[a] For PBE0-2, **6** is a clear outlier due to a strong orbital mixing in the triplet state. Removing it yields MSE, MAE, and SDE of 0.141, 0.141 and 0.045 eV, respectively.

## S2. MOS

Below we report the representation of the relevant (HF/*aug*-cc-pVTZ) molecular orbitals (MOs) for the studied transitions.

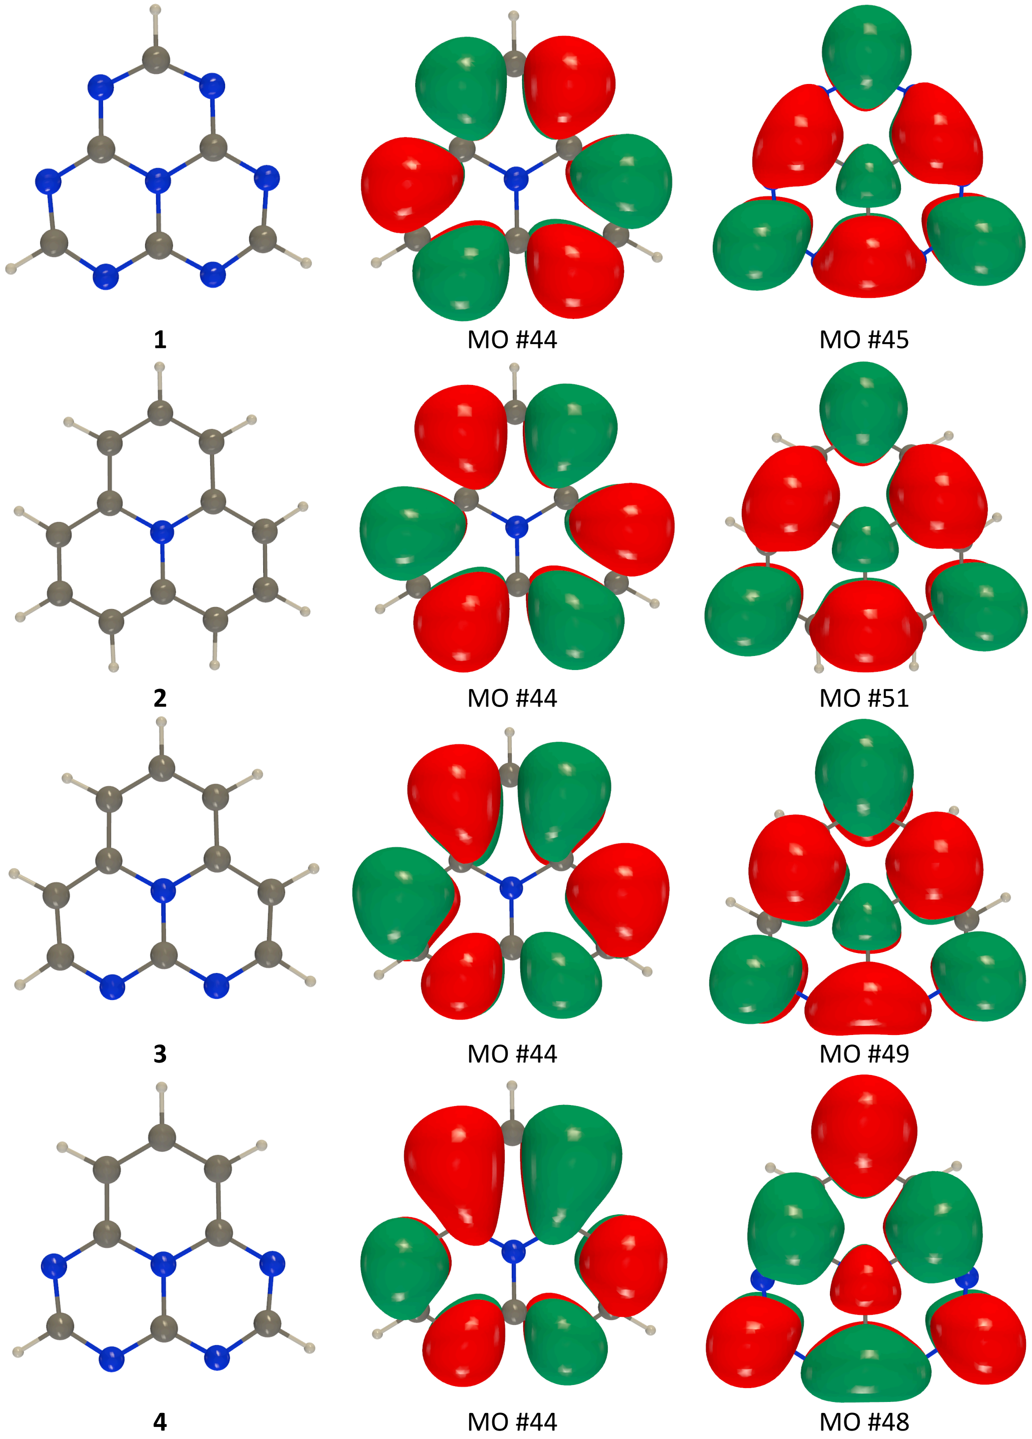


Figure S1: Key MOs for compounds **1**–**4**.

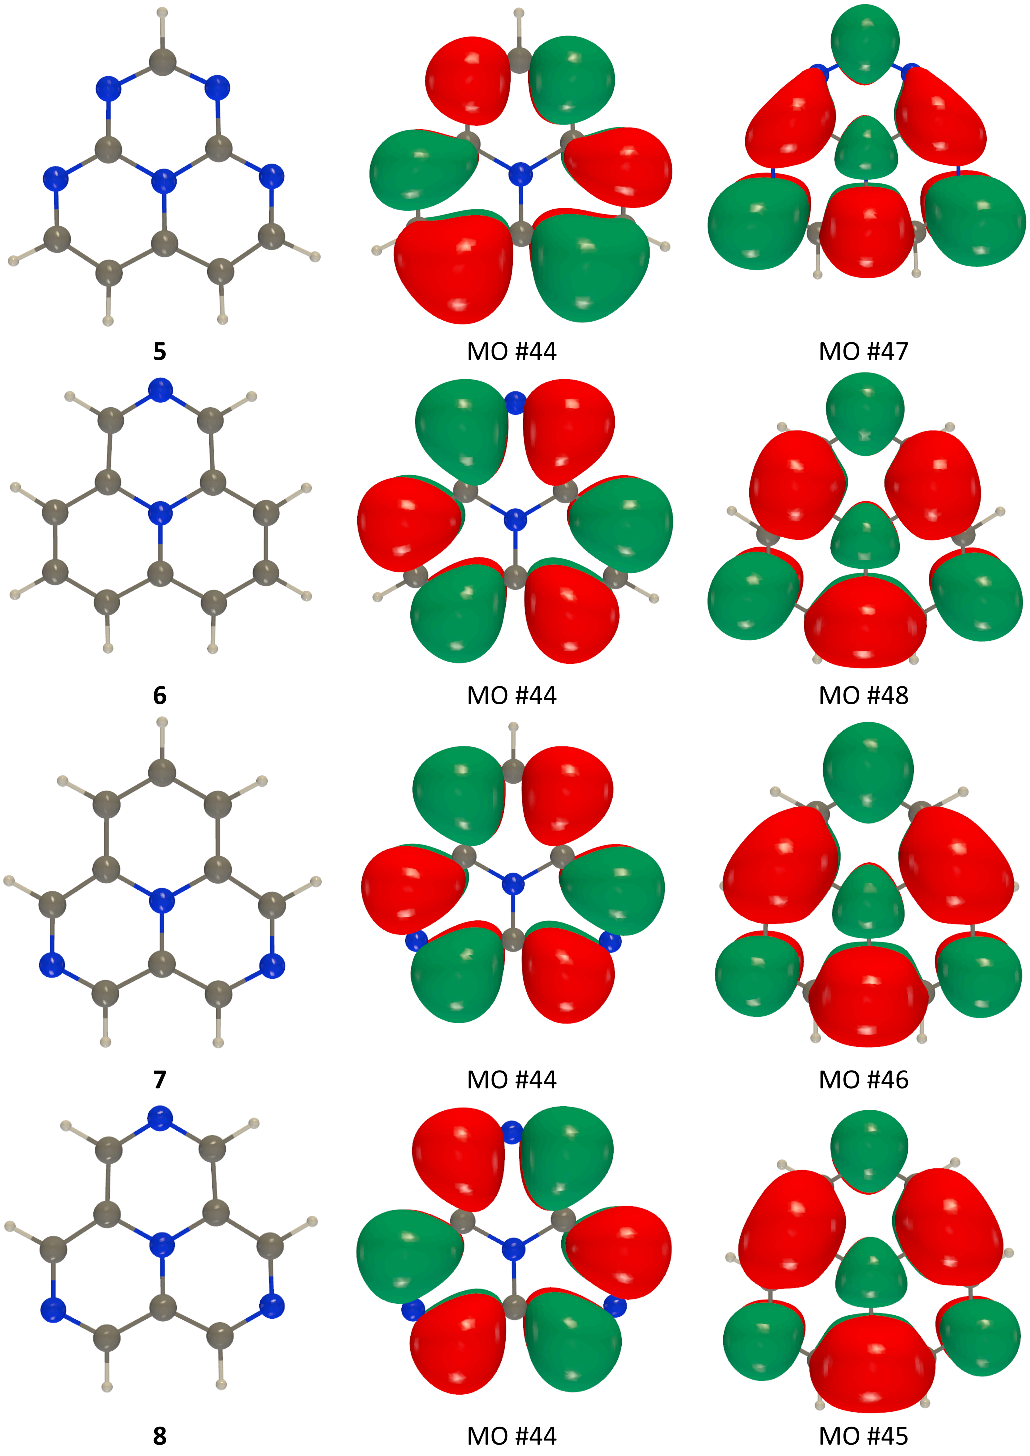


Figure S2: Key MOs for compounds **5**–**8**.

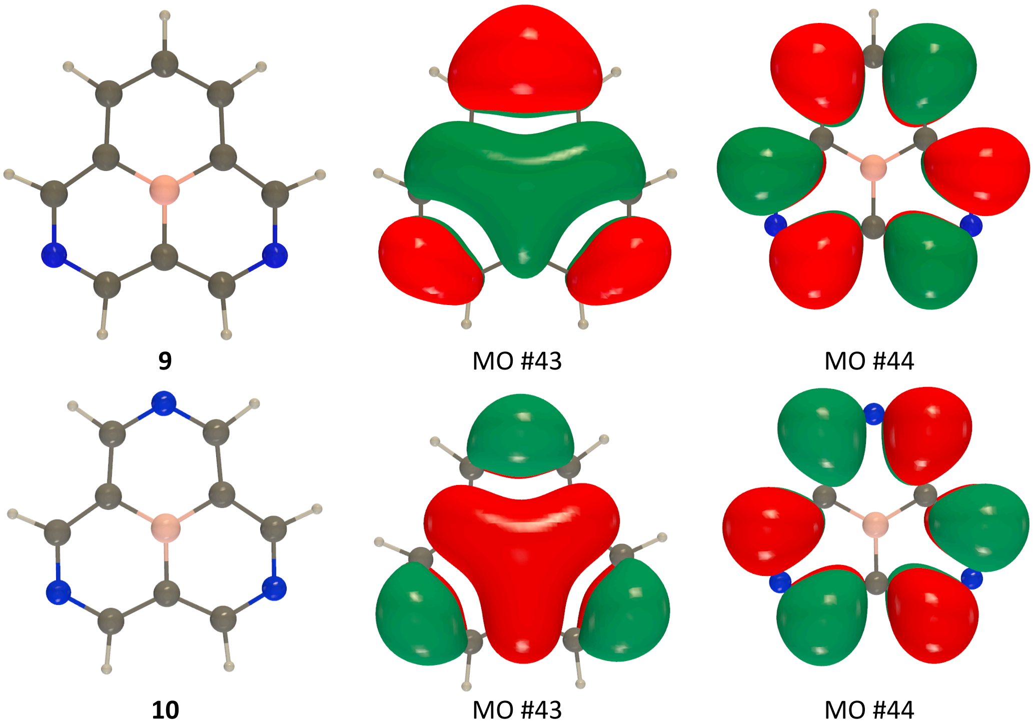


Figure S3: Key MOs for compounds **9** and **10**.

## S3. CYCLBORANE

We have also investigated cyclborane, **11**, the equivalent of cyclazine, **2** but with a central boron atom (see Figure S4). In this case, the MP2/6-311G(d,p) optimization carried out in the $D_{3h}$ point group yields an unstable structure, presenting a clear imaginary frequency ($A_2'$, $i443$ cm$^{-1}$). Deformation along this mode yields a stable $C_{3h}$ structure at the same level of theory. We have optimized **11** in both symmetries at the CCSD(T)/cc-pVTZ level, and the $C_{3h}$ structure was also found lower in energy by a small 1.07 kcal.mol$^{-1}$ value. Despite this small energetic difference, the deformation of the structure is significant (see Figure S4), with the appearance of a clear bond length alternation in the $C_{3h}$ structure.

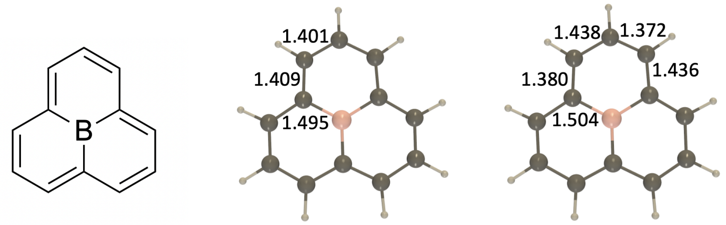


**11**
(Cyclborane) $D_{3h}$ $C_{3h}$

Figure S4: Representation of cyclborane (left), and optimal CCSD(T)/cc-pVTZ geometries obtained in the $D_{3h}$ (middle) and $C_{3h}$ (right) point groups. In the latter, all non-equivalent CC and CB distances are indicated (in Å).

In Table S6, we show the reference results obtained with ADC(2), CC2, CCSD, CC3, and CCSDT for these two structures. It appears that regardless of the selected basis set and level of theory, an inverted STG is observed in the $D_{3h}$ structure. This inversion is not found for the stable $C_{3h}$ conformer, with positive STG. Indeed, the lowering of the symmetry slightly upshifts the triplet (by approximately +0.2 eV), but strongly affects the singlet (by approximately +0.5 eV).

**Table S6: Vertical transition energies in eV for compounds 11. The numbers in parentheses are the percentages of single excitation involved in the transition computed at the CC3/aug-cc-pVDZ level.**

| | | ADC(2) | CC2 | CCSD | | | CC3 | | | CCSDT | TBE |
|---|---|---|---|---|---|---|---|---|---|---|---|
| Structure | State | AVTZ | AVTZ | 6-31+G(d) | AVDZ | AVTZ | 6-31+G(d) | AVDZ | AVTZ | 6-31+G(d) | |
| $D_{3h}$ | $S_1$ | 0.799 | 0.866 | 0.815 | 0.864 | 0.867 | 0.752 | 0.800 (86.7%) | 0.787 | 0.744 | 0.779$^a$ |
| | $T_1$ | 0.990 | 1.054 | 0.980 | 0.989 | 0.982 | 0.970 | 0.981 (95.6%) | | | 0.974$^b$ |
| $C_{3h}$ | $S_1$ | 1.262 | 1.275 | 1.424 | 1.415 | 1.420 | 1.177 | 1.179 (85.2%) | | 1.202 | 1.209$^c$ |
| | $T_1$ | 1.179 | 1.207 | 1.178 | 1.172 | 1.167 | 1.157 | 1.152 (96.4%) | | | 1.147$^b$ |

$^a$Theoretical best estimate obtained from CCSDT/6-31+G(d) + [CC3/*aug*-cc-pVTZ − CC3/6-31+G(d)]. $^b$Theoretical best estimate obtained from CC3/*aug*-cc-pVDZ + [CCSD/*aug*-cc-pVTZ − CCSD/*aug*-cc-pVDZ]. $^c$Theoretical best estimate obtained from CCSDT/6-31+G(d) + [CC3/*aug*-cc-pVDZ − CC3/6-31+G(d)] + [CCSD/*aug*-cc-pVTZ − CCSD/*aug*-cc-pVDZ].

At this stage, one can therefore conclude that it is likely that cyclborane does not present an inverted STG in its most stable conformation.

## S4. GEOMETRIES

Below are the Cartesian coordinates for all systems given in bohr.

### S4.1 Benchmark set

All geometries below are obtained at the CCSD(T)/cc-pVTZ level (within the frozen-core approximation), constraining the geometry to the highest possible point group symmetry.

S4.1.1 Molecule **1** (Heptazine)

```
C          0.00000000    -2.28707566     1.32044375
C          0.00000000    -4.25961422    -2.45928942
C          0.00000000    -0.00000000    -2.64088750
C          0.00000000     4.25961422    -2.45928942
C          0.00000000     2.28707566     1.32044375
C          0.00000000    -0.00000000     4.91857884
N          0.00000000     0.00000000    -0.00000000
N          0.00000000    -4.45372767     0.04447145
N          0.00000000     2.18835043    -3.87927703
N          0.00000000     2.26537724     3.83480558
N          0.00000000    -2.26537724     3.83480558
N          0.00000000    -2.18835043    -3.87927703
N          0.00000000     4.45372767     0.04447145
H          0.00000000     6.02612802    -3.47918663
H          0.00000000     0.00000000     6.95837327
H          0.00000000    -6.02612802    -3.47918663
```

S4.1.2 Molecule **2** (Cyclazine)

```
C          0.00000000    -2.29619838     1.32571075
C          0.00000000    -4.57380843    -2.64068953
C          0.00000000    -0.00000000    -2.65142150
C          0.00000000     4.57380843    -2.64068953
C          0.00000000     2.29619838     1.32571075
C          0.00000000     0.00000000     5.28137906
C          0.00000000    -4.57334297    -0.03501138
C          0.00000000     2.31699223    -3.94312550
C          0.00000000     2.25635074     3.97813688
C          0.00000000    -2.25635074     3.97813688
C          0.00000000    -2.31699223    -3.94312550
C          0.00000000     4.57334297    -0.03501138
N          0.00000000    -0.00000000     0.00000000
H          0.00000000     6.33829394    -3.65941571
H          0.00000000     0.00000000     7.31883143
H          0.00000000    -6.33829394    -3.65941571
```

| | | | |
|---|---|---|---|
| H | 0.00000000 | -6.29930356 | 1.03947702 |
| H | 0.00000000 | 2.24943827 | -5.97509542 |
| H | 0.00000000 | 4.04986529 | 4.93561840 |
| H | 0.00000000 | -4.04986529 | 4.93561840 |
| H | 0.00000000 | -2.24943827 | -5.97509542 |
| H | 0.00000000 | 6.29930356 | 1.03947702 |

S4.1.3 Molecule **3**

| | | | |
|---|---|---|---|
| C | 0.00000000 | -0.00000000 | 2.63044602 |
| C | 0.00000000 | 0.00000000 | -5.32562322 |
| C | 0.00000000 | -2.28292518 | -1.38006964 |
| C | 0.00000000 | 2.28292518 | -1.38006964 |
| C | 0.00000000 | -2.25969211 | -4.02080437 |
| C | 0.00000000 | 2.25969211 | -4.02080437 |
| C | 0.00000000 | -4.51358507 | 0.05853045 |
| C | 0.00000000 | 4.51358507 | 0.05853045 |
| C | 0.00000000 | -4.33214653 | 2.63970976 |
| C | 0.00000000 | 4.33214653 | 2.63970976 |
| N | 0.00000000 | -0.00000000 | -0.07278591 |
| N | 0.00000000 | -2.16002933 | 3.92349961 |
| N | 0.00000000 | 2.16002933 | 3.92349961 |
| H | 0.00000000 | -4.05303029 | -4.97864815 |
| H | 0.00000000 | 4.05303029 | -4.97864815 |
| H | 0.00000000 | -6.30224117 | -0.90474256 |
| H | 0.00000000 | 6.30224117 | -0.90474256 |
| H | 0.00000000 | -6.02602008 | 3.78110657 |
| H | 0.00000000 | 6.02602008 | 3.78110657 |
| H | 0.00000000 | 0.00000000 | -7.36246610 |

S4.1.4 Molecule **4**

| | | | |
|---|---|---|---|
| C | 0.00000000 | -0.00000000 | 2.63028268 |
| C | 0.00000000 | 0.00000000 | -5.22697144 |
| C | 0.00000000 | -2.30154257 | -1.30908237 |
| C | 0.00000000 | 2.30154257 | -1.30908237 |
| C | 0.00000000 | -2.27360261 | -3.93623932 |
| C | 0.00000000 | 2.27360261 | -3.93623932 |
| C | 0.00000000 | -4.28150962 | 2.47338977 |
| C | 0.00000000 | 4.28150962 | 2.47338977 |
| N | 0.00000000 | -0.00000000 | -0.03667172 |
| N | 0.00000000 | -4.49490929 | -0.00724176 |
| N | 0.00000000 | 4.49490929 | -0.00724176 |
| N | 0.00000000 | -2.18121748 | 3.87245554 |
| N | 0.00000000 | 2.18121748 | 3.87245554 |
| H | 0.00000000 | -4.07269227 | -4.87627993 |

| | | | |
|---|---|---|---|
| H | 0.00000000 | 4.07269227 | -4.87627993 |
| H | 0.00000000 | -6.03233631 | 3.52231827 |
| H | 0.00000000 | 6.03233631 | 3.52231827 |
| H | 0.00000000 | 0.00000000 | -7.26365004 |

S4.1.5 Molecule **5**

| | | | |
|---|---|---|---|
| C | 0.00000000 | -0.00000000 | 2.69111414 |
| C | 0.00000000 | 0.00000000 | -4.87509998 |
| C | 0.00000000 | 2.30395543 | -1.27061860 |
| C | 0.00000000 | -2.30395543 | -1.27061860 |
| C | 0.00000000 | 4.49331827 | 2.44641378 |
| C | 0.00000000 | -4.49331827 | 2.44641378 |
| C | 0.00000000 | 2.34715406 | 3.90527014 |
| C | 0.00000000 | -2.34715406 | 3.90527014 |
| N | 0.00000000 | -0.00000000 | 0.07673672 |
| N | 0.00000000 | 4.51036788 | -0.07937485 |
| N | 0.00000000 | -4.51036788 | -0.07937485 |
| N | 0.00000000 | 2.25973325 | -3.79578718 |
| N | 0.00000000 | -2.25973325 | -3.79578718 |
| H | 0.00000000 | 6.33127298 | 3.33521921 |
| H | 0.00000000 | -6.33127298 | 3.33521921 |
| H | 0.00000000 | 2.41609204 | 5.93537288 |
| H | 0.00000000 | -2.41609204 | 5.93537288 |
| H | 0.00000000 | 0.00000000 | -6.91607728 |

S4.1.6 Molecule**6**

| | | | |
|---|---|---|---|
| C | 0.00000000 | -0.00000000 | 2.69303231 |
| C | 0.00000000 | -2.26853402 | -1.29137282 |
| C | 0.00000000 | 2.26853402 | -1.29137282 |
| C | 0.00000000 | -2.13688574 | -3.95022716 |
| C | 0.00000000 | 2.13688574 | -3.95022716 |
| C | 0.00000000 | -4.56260586 | 0.02708550 |
| C | 0.00000000 | 4.56260586 | 0.02708550 |
| C | 0.00000000 | -4.57761039 | 2.63719631 |
| C | 0.00000000 | 4.57761039 | 2.63719631 |
| C | 0.00000000 | -2.33218960 | 3.96312458 |
| C | 0.00000000 | 2.33218960 | 3.96312458 |
| N | 0.00000000 | -0.00000000 | 0.05321330 |
| N | 0.00000000 | 0.00000000 | -5.25366390 |
| H | 0.00000000 | -3.89456715 | -4.98070200 |
| H | 0.00000000 | 3.89456715 | -4.98070200 |
| H | 0.00000000 | -6.27773451 | -1.06394342 |
| H | 0.00000000 | 6.27773451 | -1.06394342 |
| H | 0.00000000 | -6.34863038 | 3.64400469 |

| | | | |
|---|---|---|---|
| H | 0.00000000 | 6.34863038 | 3.64400469 |
| H | 0.00000000 | -2.28865346 | 5.99578516 |
| H | 0.00000000 | 2.28865346 | 5.99578516 |

S4.1.7 Molecule **7**

| | | | |
|---|---|---|---|
| C | 0.00000000 | -0.00000000 | 2.57288762 |
| C | 0.00000000 | 0.00000000 | -5.28547533 |
| C | 0.00000000 | 2.28819776 | -1.33986473 |
| C | 0.00000000 | -2.28819776 | -1.33986473 |
| C | 0.00000000 | 2.34330473 | 3.82174697 |
| C | 0.00000000 | -2.34330473 | 3.82174697 |
| C | 0.00000000 | 2.26733906 | -3.98866184 |
| C | 0.00000000 | -2.26733906 | -3.98866184 |
| C | 0.00000000 | 4.51483069 | 0.12733957 |
| C | 0.00000000 | -4.51483069 | 0.12733957 |
| N | 0.00000000 | 4.54965666 | 2.63028556 |
| N | 0.00000000 | -0.00000000 | -0.05181144 |
| N | 0.00000000 | -4.54965666 | 2.63028556 |
| H | 0.00000000 | 0.00000000 | -7.32242747 |
| H | 0.00000000 | 2.34321313 | 5.85832928 |
| H | 0.00000000 | -2.34321313 | 5.85832928 |
| H | 0.00000000 | 6.29748236 | -0.85930252 |
| H | 0.00000000 | -6.29748236 | -0.85930252 |
| H | 0.00000000 | 4.05836778 | -4.95006415 |
| H | 0.00000000 | -4.05836778 | -4.95006415 |

S4.1.8 Molecule **8**

| | | | |
|---|---|---|---|
| C | 0.00000000 | -2.26352511 | 1.30684683 |
| C | 0.00000000 | -0.00000000 | -2.61369367 |
| C | 0.00000000 | 2.26352511 | 1.30684683 |
| C | 0.00000000 | -4.50716704 | -0.12180998 |
| C | 0.00000000 | 2.35907406 | -3.84241616 |
| C | 0.00000000 | 2.14809298 | 3.96422614 |
| C | 0.00000000 | -2.14809298 | 3.96422614 |
| C | 0.00000000 | -2.35907406 | -3.84241616 |
| C | 0.00000000 | 4.50716704 | -0.12180998 |
| N | 0.00000000 | -0.00000000 | 0.00000000 |
| N | 0.00000000 | -4.55331317 | -2.62885659 |
| N | 0.00000000 | 4.55331317 | -2.62885659 |
| N | 0.00000000 | 0.00000000 | 5.25771317 |
| H | 0.00000000 | -6.28226830 | 0.87641508 |
| H | 0.00000000 | 2.38213643 | -5.87881148 |
| H | 0.00000000 | 3.90013187 | 5.00239640 |
| H | 0.00000000 | -3.90013187 | 5.00239640 |

| | | | |
|---|---|---|---|
| H | 0.00000000 | -2.38213643 | -5.87881148 |
| H | 0.00000000 | 6.28226830 | 0.87641508 |

S4.1.9 Molecule **9**

| | | | |
|---|---|---|---|
| B | 0.00000000 | 0.00000000 | -0.05273140 |
| C | 0.00000000 | 0.00000000 | 2.74223189 |
| C | 0.00000000 | 0.00000000 | -5.33744297 |
| C | 0.00000000 | 2.45002887 | -1.42250939 |
| C | 0.00000000 | -2.45002887 | -1.42250939 |
| C | 0.00000000 | 2.38780296 | 3.90963736 |
| C | 0.00000000 | -2.38780296 | 3.90963736 |
| C | 0.00000000 | 2.33669736 | -4.08087398 |
| C | 0.00000000 | -2.33669736 | -4.08087398 |
| C | 0.00000000 | 4.61478223 | 0.11491651 |
| C | 0.00000000 | -4.61478223 | 0.11491651 |
| N | 0.00000000 | 4.60210444 | 2.66349182 |
| N | 0.00000000 | -4.60210444 | 2.66349182 |
| H | 0.00000000 | 0.00000000 | -7.37464827 |
| H | 0.00000000 | 2.57750127 | 5.95330533 |
| H | 0.00000000 | -2.57750127 | 5.95330533 |
| H | 0.00000000 | 6.49745564 | -0.70393848 |
| H | 0.00000000 | -6.49745564 | -0.70393848 |
| H | 0.00000000 | 4.03886143 | -5.22298037 |
| H | 0.00000000 | -4.03886143 | -5.22298037 |

S4.1.10 Molecule **10**

| | | | |
|---|---|---|---|
| B | 0.00000000 | -0.00000000 | 0.00000000 |
| C | 0.00000000 | -2.41881246 | 1.39650203 |
| C | 0.00000000 | -0.00000000 | -2.79300406 |
| C | 0.00000000 | 2.41881246 | 1.39650203 |
| C | 0.00000000 | -4.60570992 | -0.11146995 |
| C | 0.00000000 | 2.39939076 | -3.93292682 |
| C | 0.00000000 | 2.20631915 | 4.04439677 |
| C | 0.00000000 | -2.20631915 | 4.04439677 |
| C | 0.00000000 | -2.39939076 | -3.93292682 |
| C | 0.00000000 | 4.60570992 | -0.11146995 |
| N | 0.00000000 | -4.60311804 | -2.65761144 |
| N | 0.00000000 | 4.60311804 | -2.65761144 |
| N | 0.00000000 | 0.00000000 | 5.31522288 |
| H | 0.00000000 | -6.48246078 | 0.71791171 |
| H | 0.00000000 | 2.61950061 | -5.97293157 |
| H | 0.00000000 | 3.86296017 | 5.25501986 |
| H | 0.00000000 | -3.86296017 | 5.25501986 |
| H | 0.00000000 | -2.61950061 | -5.97293157 |

| | | | |
|---|---|---|---|
| H | 0.00000000 | 6.48246078 | 0.71791171 |

**S4.2 0-0 energy calculations of heptazine**

The geometries below have been obtained with CCSD/cc-pVDZ ($S_0$), EOM-CCSD/cc-pVDZ ($S_1$), and UCCSD/cc-pVDZ ($T_1$). They are all true minima at their respective level of theory. The frozen-core approximation was enforced. As explained in the main text, two minima are obtained for the triplet state when one starts from the fully symmetric $D_{3h}$ geometry.

S4.2.1 Ground state ($D_{3h}$)

| | | | |
|---|---|---|---|
| C | 0.00000000 | 2.65843295 | 0.00000000 |
| C | -4.28260596 | 2.47256323 | 0.00000000 |
| C | -2.30227083 | -1.32921693 | 0.00000000 |
| C | 0.00000000 | -4.94512737 | 0.00000000 |
| C | 2.30227083 | -1.32921693 | 0.00000000 |
| C | 4.28260596 | 2.47256323 | 0.00000000 |
| N | 0.00000000 | -0.00000031 | 0.00000000 |
| N | -2.20315656 | 3.91218524 | 0.00000000 |
| N | -2.28647271 | -3.86408097 | 0.00000000 |
| N | 4.48962928 | -0.04810329 | 0.00000000 |
| N | 2.20315656 | 3.91218524 | 0.00000000 |
| N | -4.48962928 | -0.04810329 | 0.00000000 |
| N | 2.28647271 | -3.86408097 | 0.00000000 |
| H | 0.00000000 | -7.01858066 | 0.00000000 |
| H | 6.07826945 | 3.50928987 | 0.00000000 |
| H | -6.07826945 | 3.50928987 | 0.00000000 |

S4.2.2 Singlet excited state ($C_{3v}$)

| | | | |
|---|---|---|---|
| C | 1.33057345 | 0.07205441 | 2.30461976 |
| C | 4.98496628 | -0.03995157 | 0.00000000 |
| C | 1.33057345 | 0.07205441 | -2.30461976 |
| C | -2.49248314 | -0.03995157 | -4.31710858 |
| C | -2.66114690 | 0.07205441 | 0.00000000 |
| C | -2.49248314 | -0.03995157 | 4.31710858 |
| N | 0.00000000 | 0.50986059 | 0.00000000 |
| N | 3.85065416 | -0.09556244 | 2.29079263 |
| N | 0.05855696 | -0.09556244 | -4.48016175 |
| N | -3.90921111 | -0.09556244 | 2.18936912 |
| N | 0.05855696 | -0.09556244 | 4.48016175 |
| N | 3.85065416 | -0.09556244 | -2.29079263 |
| N | -3.90921111 | -0.09556244 | -2.18936912 |
| H | -3.52603883 | -0.08808101 | -6.10727864 |

| | | | |
|---|---|---|---|
| H | -3.52603883 | -0.08808101 | 6.10727864 |
| H | 7.05207765 | -0.08808101 | 0.00000000 |

S4.2.3 Triplet excited state ($C_{3v}$)

| | | | |
|---|---|---|---|
| C | 1.33389005 | 0.05479459 | 2.31036642 |
| C | 4.98701676 | -0.03181158 | 0.00000000 |
| C | 1.33389005 | 0.05479459 | -2.31036642 |
| C | -2.49350913 | -0.03181157 | -4.31888304 |
| C | -2.66777971 | 0.05479459 | 0.00000000 |
| C | -2.49350913 | -0.03181157 | 4.31888304 |
| N | 0.00000013 | 0.37577409 | 0.00000000 |
| N | 3.85405769 | -0.06973272 | 2.29223638 |
| N | 0.05810544 | -0.06973272 | -4.48382970 |
| N | -3.91216273 | -0.06973271 | 2.19159521 |
| N | 0.05810544 | -0.06973272 | 4.48382970 |
| N | 3.85405769 | -0.06973272 | -2.29223638 |
| N | -3.91216273 | -0.06973271 | -2.19159521 |
| H | -3.52652624 | -0.07625227 | -6.10812335 |
| H | -3.52652624 | -0.07625227 | 6.10812335 |
| H | 7.05305288 | -0.07625228 | 0.00000000 |

S4.2.4 Triplet excited state ($C_s$)

| | | | |
|---|---|---|---|
| C | 2.58131049 | -0.77032087 | 0.00000000 |
| C | 1.25597608 | -4.87176503 | 0.00000000 |
| C | -1.89359322 | -1.88862106 | 0.00000000 |
| C | -4.80791262 | 1.34882018 | 0.00000000 |
| C | -0.62544766 | 2.55285192 | 0.00000000 |
| C | 3.62956701 | 3.43349485 | 0.00000000 |
| N | -0.01094162 | 0.01903881 | 0.00000000 |
| N | 3.15733943 | -3.18472630 | 0.00000000 |
| N | -4.39487960 | -1.11493986 | 0.00000000 |
| N | 1.13864801 | 4.34332697 | 0.00000000 |
| N | 4.40331772 | 1.09474027 | 0.00000000 |
| N | -1.32660891 | -4.27133170 | 0.00000000 |
| N | -3.08767133 | 3.28229927 | 0.00000000 |
| H | -6.79016061 | 1.94934022 | 0.00000000 |
| H | 5.07367966 | 4.91624323 | 0.00000000 |
| H | 1.72910074 | -6.87723406 | 0.00000000 |

### S4.3 Cyclborane

Below are the GS geometries obtained at the CCSD(T)/cc-pVTZ level (FC applied) for cyclborane, **11**. The $D_{3h}$ structure is less stable than the $C_{3h}$ one by 1.07 kcal.mol$^{-1}$ at this level of theory. We note that

MP2/6-311G(d,p) returns an imaginary frequency for the former, but none for the latter (considering the MP2/6-311G(d,p) optimal structures of course).

S4.3.1 Ground state ($D_{3h}$)

| | | | |
|---|---|---|---|
| B | 0.00000000 | -0.00000000 | 0.00000000 |
| C | 0.00000000 | -2.44612494 | 1.41227089 |
| C | 0.00000000 | -4.62663758 | -2.67119045 |
| C | 0.00000000 | -0.00000000 | -2.82454179 |
| C | 0.00000000 | 4.62663758 | -2.67119045 |
| C | 0.00000000 | 2.44612494 | 1.41227089 |
| C | 0.00000000 | 0.00000000 | 5.34238090 |
| C | 0.00000000 | -4.68824151 | -0.02387497 |
| C | 0.00000000 | 2.36479709 | -4.04819876 |
| C | 0.00000000 | 2.32344442 | 4.07207374 |
| C | 0.00000000 | -2.32344442 | 4.07207374 |
| C | 0.00000000 | -2.36479709 | -4.04819876 |
| C | 0.00000000 | 4.68824151 | -0.02387497 |
| H | 0.00000000 | 6.39092881 | -3.68980447 |
| H | 0.00000000 | 0.00000000 | 7.37960894 |
| H | 0.00000000 | -6.39092881 | -3.68980447 |
| H | 0.00000000 | -6.52257542 | 0.89376489 |
| H | 0.00000000 | 2.48726461 | -6.09559846 |
| H | 0.00000000 | 4.03531081 | 5.20183357 |
| H | 0.00000000 | -4.03531081 | 5.20183357 |
| H | 0.00000000 | -2.48726461 | -6.09559846 |
| H | 0.00000000 | 6.52257542 | 0.89376489 |

S4.3.2 Ground state ($C_{3h}$)

| | | | |
|---|---|---|---|
| B | 0.00000000 | 0.00000000 | -0.00000000 |
| C | -2.44037550 | -1.45845179 | -0.00000000 |
| C | 2.48324406 | -1.38420128 | -0.00000000 |
| C | -0.04286855 | 2.84265308 | 0.00000000 |
| C | -4.64032868 | -0.05832113 | 0.00000000 |
| C | 2.37067192 | -3.98948196 | -0.00000000 |
| C | 2.26965676 | 4.04780308 | 0.00000000 |
| C | -4.63652241 | 2.65836628 | 0.00000000 |
| C | 0.01604847 | -5.34452933 | -0.00000000 |
| C | 4.62047394 | 2.68616305 | 0.00000000 |
| C | -2.46300234 | 4.07079265 | 0.00000000 |
| C | -2.29390868 | -4.16841893 | -0.00000000 |
| C | 4.75691102 | 0.09762627 | -0.00000000 |
| H | -6.47241079 | -0.98272907 | 0.00000000 |
| H | 4.08727374 | -5.11390763 | -0.00000000 |
| H | 2.38513705 | 6.09663670 | 0.00000000 |

| | | | |
|---|---|---|---|
| H | -6.43994442 | 3.60709504 | 0.00000000 |
| H | 0.09613627 | -7.38070299 | -0.00000000 |
| H | 6.34380815 | 3.77360795 | 0.00000000 |
| H | -2.60335046 | 6.11370892 | 0.00000000 |
| H | -3.99295201 | -5.31142209 | -0.00000000 |
| H | 6.59630247 | -0.80228683 | -0.00000000 |
